# Supplementary material for: AgenticRec: A Recommendation-Oriented Agentic Framework with Progressive Tool-Integrated Reasoning Optimization
Source: arXiv:2603.21613 source file (2026-06-14)
Supplement: Supplementary file 1 [file Theoretical_Analysis_v2.tex]

% 下面是正文中对应理论分析的部分，将作为方法介绍章节的最后一个subsection出现。
% 该部分的作用是简单概括我们得到了两个proposition，点出其作为对两阶段训练目标的合理性解释（而非性能保证），并说明具体内容详见附录。
% \subsection{Theoretical Justifications}
% We provide theoretical justifications interpreting why both training stages of \ours are well-aligned with their recommendation objectives, rather than offering performance guarantees. Specifically,
% (1) with a stop-gradient inclusive group-average baseline, the RTA gradient estimator is directionally aligned with the policy gradient of the expected list-wise utility objective (i.e., NDCG@K), supporting credit propagation over tool-integrated trajectories;
% (2) under a pairwise softmax approximation, the PPR objective on mined hard pairs minimizes a logistic surrogate upper bound of the pair-wise misordering loss, thereby sharpening fine-grained preference boundaries.
% Together, these results indicate that the two stages of \ours are theoretically sound and jointly contribute to the final result. Formal statements and proofs are deferred to Appendix~\ref{app:theoretical_analysis}.

\section{Theoretical Analysis}
\label{app:theoretical_analysis}

\subsection{Directional Alignment of the RTA Gradient}
\label{app:unbias}

Under standard conditions on the rollout procedure, the RTA gradient estimator remains directionally aligned with the policy gradient of the shaped list-wise reward objective, up to a positive scaling factor:
\begin{proposition}[Directional Alignment of the RTA Gradient]
\label{prop:unbias}
    Assume independent rollouts $\{\tau^{(g)}\}_{g=1}^{G}$ ($G>1$) drawn from $\pi_\theta$ and a stop-gradient inclusive group-average baseline, and consider the population estimator (i.e., without clipping, advantage normalization, or dynamic filtering). Then the RTA gradient estimator that uses the shaped list-wise reward $R(r_K, y)$ defined in Eq.~\ref{eq:main_reward} as the reward signal and the inclusive group-average ranking score as the baseline provides a directionally aligned estimate of the gradient of the expected shaped list-wise reward objective $J(\theta) = \mathbb{E}_{\tau \sim \pi_\theta}[R(r_K, y)]$, up to the positive scaling factor $\frac{G-1}{G}$.
\end{proposition} 
Proposition~\ref{prop:unbias} states that the computed gradient direction aligns with the policy gradient of the expected shaped list-wise reward objective $J(\theta)$, which is anchored by the recommendation reward $R_{\text{rec}}$ (NDCG@K, Eq.~\ref{eq:rankreward}) and additionally shaped by the validity and tool-use components in Eq.~\ref{eq:main_reward}. The inclusive baseline introduces only a positive scaling factor $\frac{G-1}{G}$ when $G>1$, which acts as a learning-rate dampener without altering the optimization direction. This directional alignment is meaningful for \ours in two ways: (1) First, it supports \emph{trajectory-level} credit propagation over reasoning and tool-use traces: a high list-wise reward jointly increases the log-probability of the entire trajectory, so that productive reasoning and tool-use patterns are reinforced as a whole. We do not claim accurate fine-grained, step-level credit assignment to individual tool calls, which we leave as a promising future direction. (2) Second, it provides stability in sparse-feedback environments: anchoring the gradient update to a group baseline focuses optimization on relative list improvement rather than unstable absolute scores, which is helpful when learning from noisy implicit ranking signals.

\begin{proof}
In \ours, the optimization goal is to maximize the expected shaped list-wise reward of the generated top-$K$ list $r_K$ given user context $x_u$. The trajectory $\tau$ encompasses the entire reasoning chain, including tool invocations (Act) and observations (Obs), culminating in the final ranking action $r_K$. By the policy-gradient identity, the gradient of the objective is:
\begin{equation}
\nabla J(\theta) = \mathbb{E}_{\tau \sim \pi_\theta} [R(r_K, y) \cdot \nabla \log \pi_\theta(\tau)],
\end{equation}
where $R(r_K, y)$ is the shaped list-wise reward in Eq.~\ref{eq:main_reward}, anchored by the recommendation reward $R_{\text{rec}}$ (NDCG@K, Eq.~\ref{eq:rankreward}) and modulated by the validity and tool-use shaping terms.

To address the high variance inherent in list-wise ranking rewards, we employ the GRPO estimator using a group of $G$ sampled trajectories $\{\tau^{(g)}\}_{g=1}^G$. The estimated gradient is:
\begin{equation}
\begin{aligned}
        \nabla \hat{J}_{GRPO}(\theta) &= \frac{1}{G} \sum_{g=1}^{G} \\
        &(R(r_K^{(g)}, y) - b) \nabla \log \pi_\theta(\tau^{(g)})
\end{aligned}
\end{equation}
where the baseline $b = \frac{1}{G} \sum_{j=1}^G R(r_K^{(j)}, y)$ is the average list-wise utility of the sampled group.

With the inclusive group-average baseline, the baseline term does not vanish exactly because $b$ contains the reward of the same trajectory $\tau^{(g)}$. Let $R^{(g)}=R(r_K^{(g)}, y)$ and $z^{(g)}=\nabla \log \pi_\theta(\tau^{(g)})$. Using the likelihood ratio identity, we have:
\begin{equation}
    \label{eq:baseline}
    \resizebox{\linewidth}{!}{$
    \begin{aligned}
        \mathbb{E}_{\tau} [\nabla \log \pi_\theta(\tau)] &= \int \pi_\theta(\tau) \cdot \nabla \log \pi_\theta(\tau) \, d\tau \\
        &= \int \pi_\theta(\tau) \cdot \frac{\nabla \pi_\theta(\tau)}{\pi_\theta(\tau)} \, d\tau \\
        &= \int \nabla \pi_\theta(\tau) \, d\tau \\
        &= \nabla \left( \int \pi_\theta(\tau) \, d\tau \right) \\
        &= \nabla (1) = 0,
    \end{aligned}
    $}
\end{equation}
where $\int \pi_\theta(\tau) \, d\tau = 1$ since the integral of any probability distribution over its entire domain must sum to 1.

Therefore, for each $g$,
\begin{equation}
\resizebox{\linewidth}{!}{$
\begin{aligned}
\mathbb{E}[b \cdot z^{(g)}]
&= \mathbb{E}\left[\frac{1}{G}\sum_{j=1}^{G} R^{(j)} z^{(g)}\right] \\
&= \frac{1}{G}\mathbb{E}[R^{(g)} z^{(g)}] + \frac{1}{G}\sum_{j\neq g}\mathbb{E}[R^{(j)}]\mathbb{E}[z^{(g)}] \\
&= \frac{1}{G}\nabla J(\theta).
\end{aligned}
$}
\end{equation}
It follows that
\begin{equation}
\resizebox{\linewidth}{!}{$
\begin{aligned}
\mathbb{E}[\nabla \hat{J}_{GRPO}(\theta)]
&= \frac{1}{G}\sum_{g=1}^{G}\left(\mathbb{E}[R^{(g)}z^{(g)}]-\mathbb{E}[b z^{(g)}]\right) \\
&= \left(1-\frac{1}{G}\right)\nabla J(\theta) \\
&= \frac{G-1}{G}\nabla J(\theta).
\end{aligned}
$}
\end{equation}
Since $G>1$, $\frac{G-1}{G}$ is strictly positive. Therefore, the expected GRPO estimator points along the same direction as $\nabla J(\theta)$, the policy gradient of the shaped list-wise reward objective anchored by NDCG@K, while the group-relative subtraction $(R^{(g)} - b)$ reduces variance by focusing on the relative ranking quality within the group.
\end{proof}

Proposition~\ref{prop:unbias} characterizes the unfiltered rollout estimator under the shaped list-wise reward $R(r_K, y)$ in Eq.~\ref{eq:main_reward}, where the format penalty, miss penalty, and tool-call bonus are absorbed into $R$ as trajectory-conditioned offsets; the directional-alignment argument above is agnostic to such offsets as long as they enter through the scalar reward. In practice, however, \ours additionally employs (i) dynamic sampling that drops rollout groups in which all sampled trajectories receive negative rewards, and may further employ (ii) PPO-style clipping and advantage normalization within GRPO. Dynamic sampling effectively conditions the update on the event that the rollout group is informative, which corresponds to optimizing a conditional objective over informative groups rather than the unconditional $J(\theta)$, and is used as a practical variance-reduction and curriculum strategy. Clipping and normalization further deviate from the population estimator. Consequently, Proposition~\ref{prop:unbias} should be read as a sanity check on the unfiltered estimator rather than as a strict guarantee over the full training pipeline.

\subsection{A Pairwise Logistic Surrogate View of Bidirectional Preference Reasoning}
\label{app:bidirectional}

The bidirectional preference reasoning in the PPR stage admits a pairwise-surrogate interpretation that motivates its potential to sharpen fine-grained preference boundaries on hard pairs:
\begin{proposition}[Pairwise Logistic Surrogate Bound for Bidirectional Preference Reasoning]
\label{prop:bidirectional}
    Let $s_\theta(c\mid x_u)$ denote the implicit pairwise preference score induced by the agent on a paired-choice PPR query (e.g., derived from the agent's answer log-probability), and let $\Delta s = s_\theta(c^+\mid x_u)-s_\theta(c^-\mid x_u)$. Under a pairwise softmax approximation of the agent-induced preference distribution, the bidirectional preference reasoning objective on mined hard pseudo-pairs $(c^+, c^-)$ corresponds to minimizing a logistic surrogate $\mathcal{L}_{Bi}(\Delta s) = 2\log(1+e^{-\Delta s})$ that upper-bounds the pairwise 0--1 misordering loss $\mathbb{I}(\Delta s < 0)$ with respect to the score margin $\Delta s$.
\end{proposition} 
Proposition~\ref{prop:bidirectional} provides an interpretation rather than a strict guarantee: by training on mined ranking violations (where initially $\Delta s < 0$), PPR optimizes a smooth convex (in $\Delta s$) surrogate of the pairwise misordering loss, which encourages enlarging the score margin between $c^+$ and $c^-$ on hard pairs. Under the scalar-score abstraction, the positive and negative directions reinforce the \emph{same} margin and therefore amount to doubling the surrogate penalty on misordered hard pairs; the proposition itself does not prove that bidirectional reasoning is mathematically more informative than a positive-only baseline at the score level. The practical benefit of bidirectional reasoning instead arises from the \emph{direction-specific prompts} in our implementation (Sec.~\ref{sec:ppr}): the positive direction encourages reasoning about matching evidence for $c^+$, while the negative direction encourages reasoning about rejection evidence for $c^-$, providing complementary linguistic supervision that the scalar-score abstraction does not fully capture.

\begin{proof}
For analysis, we view the agent as inducing an implicit pairwise preference score $s_\theta(c\mid x_u)$ over candidate items---for example, derived from the agent's answer log-probability on the paired-choice PPR query. This abstraction is used only to interpret the refinement signal at the score level, and is not intended to fully characterize the LLM trajectory distribution. We use $s(c)$ as shorthand for $s_\theta(c\mid x_u)$ when there is no ambiguity. Following the standard implicit-feedback convention, we treat mined competitors $c^-$ as \emph{pseudo} hard-negative items rather than verified dispreferred items.

A pairwise ranking violation occurs if $s(c^-) > s(c^+)$ for a mined competitor $c^-$. We define the score margin as
\begin{equation}
    \Delta s = s(c^+) - s(c^-),
\end{equation}
so that a pairwise misordering corresponds to $\Delta s < 0$.

A direct goal of pairwise ranking optimization is to minimize the misordering rate, given by the indicator
\begin{equation}
    \mathcal{L}_{0-1}(\Delta s) = \mathbb{I}(\Delta s < 0) = \begin{cases} 1 & \text{if } \Delta s < 0, \\ 0 & \text{if } \Delta s \ge 0. \end{cases}
\end{equation}
Directly optimizing $\mathcal{L}_{0-1}$ is intractable due to its discontinuity and zero gradients almost everywhere, which prevents effective gradient-based updates of the agent's policy.

For a pair $(c^+, c^-)$, our bidirectional preference reasoning creates two complementary tasks. Under a \emph{pairwise softmax approximation} of the agent-induced preference distribution---i.e., treating the agent's choice probability between the two candidates as a softmax over the induced scores $\{s(c^+), s(c^-)\}$---we have:
\begin{itemize}[leftmargin=10pt,topsep=3pt,itemsep=0.2pt]
    \item \textbf{Positive Direction:} Maximize likelihood of choosing $c^+$. Under the pairwise softmax, this probability is 
    $$P_{pos} = \frac{e^{s(c^+)}}{e^{s(c^+)} + e^{s(c^-)}}.$$
    
    \item \textbf{Negative Direction:} Maximize likelihood of rejecting $c^-$ (identifying it as ``less likely''), which under the same pairwise softmax view amounts to maximizing
    $$P_{neg} = \frac{e^{-s(c^-)}}{e^{-s(c^+)} + e^{-s(c^-)}} = \frac{e^{s(c^+)}}{e^{s(c^+)} + e^{s(c^-)}}.$$
    Notably, $P_{neg}=P_{pos}$ under the scalar-score abstraction, so the two directions reinforce the same pairwise margin (we discuss the implications below).
\end{itemize}

Under this pairwise softmax approximation, optimizing each direction with the binary correctness reward via GRPO can be interpreted as minimizing the negative log-likelihood (cross-entropy) of the corresponding preference probability $P(c^+\succ c^-)$, up to standard simplifications on the policy parameterization (e.g., neglecting clipping, advantage normalization, and entropy regularization). We do \emph{not} claim a strict equivalence between the GRPO update and a supervised cross-entropy loss; rather, the cross-entropy form serves as an interpretable surrogate for the induced pairwise objective.

For the pair $(c^+, c^-)$, the combined surrogate loss $\mathcal{L}_{Bi}$ is then proportional to:
\begin{equation}
\begin{aligned}
    \mathcal{L}_{Bi} &\approx - \log(P_{pos}) - \log(P_{neg}) \\
    &= - 2 \log \left( \frac{1}{1 + e^{-(s(c^+) - s(c^-))}} \right) \\
    &= 2\log(1 + e^{-\Delta s}).
\end{aligned}
\end{equation}
The above formulation represents the logistic loss.

The derived logistic loss $\mathcal{L}(\Delta s) = 2\log(1 + e^{-\Delta s})$ serves as a surrogate upper bound (in $\Delta s$) to the 0--1 misordering loss $\mathcal{L}_{0-1}$:
\begin{itemize}[leftmargin=10pt,topsep=5pt,itemsep=0.2pt]
    \item \textbf{Surrogate Upper Bound (in $\Delta s$):} For any $\Delta s$, $2\log(1 + e^{-\Delta s}) \ge 2\log(2)\cdot\mathbb{I}(\Delta s < 0)$. When $\Delta s < 0$ (a misordering), the logistic loss grows approximately linearly in $-\Delta s$, imposing an increasing penalty; when $\Delta s > 0$ (correct ordering), the loss approaches zero smoothly. We note that this is a valid surrogate upper bound up to the constant $2\log 2$, rather than a tight bound at every point.

    \item \textbf{Convex in the Margin (but not in $\theta$):} Unlike the step function $\mathbb{I}(\cdot)$, the logistic loss $\mathcal{L}(\Delta s)$ is smooth and convex \emph{in the margin $\Delta s$}, providing non-vanishing gradients with respect to $\Delta s$ even when the ranking is currently incorrect ($\Delta s\ll 0$). This convexity is in the score margin, \emph{not} in the LLM parameters $\theta$; the actual optimization over $\theta$ remains non-convex, so the surrogate does not imply a globally convex training landscape.
\end{itemize}

By mining hard pseudo-negatives where $\Delta s < 0$ and applying the bidirectional update, \ours minimizes the surrogate $2\log(1 + e^{-\Delta s})$ with respect to the margin. Because this surrogate provides a smooth convex (in $\Delta s$) upper bound of the pairwise misordering indicator, optimizing it encourages reducing the empirical pairwise misordering rate on mined hard pairs, thereby sharpening the fine-grained preference boundaries among highly confusable candidates. We emphasize that this does not constitute a global optimization guarantee for the non-convex LLM policy; rather, it offers a principled surrogate-minimization interpretation of PPR.
\end{proof}
